# Supplementary material for: Text-CRS: A Generalized Certified Robustness Framework against Textual Adversarial Attacks
Source: arXiv:2307.16630 source file (2024-06-11)
Supplement: Supplementary file 1 [file appendix_m.tex]

\appendix

%%%%%%%%%%%%%%%%%%%%%%%%%%%%%%%%%%%%%%%%%%%%%%%%%%%%%%%%%%%%%%%%%%%%%%%%%%
\subsection{Proof for Theorem~\ref{thm:wss_1} (binary case)} \label{proof:wss_2}

\begin{definition} (Constrained Adversarial Certification) We first define
\begin{equation}
    \min_{\delta\in\CB} h^\sharp_{\pi_0}(x_0+\delta) = \min_{\delta\in \CB}\BE_{z\sim \pi_0}[h^\sharp(x_0+z+\delta)]
\end{equation}
we assume $\CH$ is a function class which is known to include $h^\sharp$, then we have 
\begin{equation}
\begin{aligned}
\label{eq:cac}
    & \min_{\delta\in\CB} h^\sharp_{\pi_0}(x_0+\delta) \\
    \geq & \min_{h\in \CH} \max_{\delta\in \CB} \{h_{\pi_0}(x_0+\delta) \mathrm{\ s.t.\ } h_{\pi_\delta}(x_0)=h^\sharp_{\pi_0}(x_0)\}
\end{aligned}
\end{equation}
\end{definition}

\begin{theorem} [Functional Optimization Bound~\cite{zhang2020black}] 
Denote the lower bound of Eq.(\ref{eq:cac}) as $\CL_{\pi_0}(\CH,\CB)$. Denote the distribution of $z+\delta$ when $z \sim \pi_0$ as $\pi_\delta$. Assume $\CH$ and $\CB$ are compact sets. We can rewrite the lower bound of $\CL_{\pi_0}(\CH,\CB)$ following minimax form using the Lagrangian function as
\begin{equation}
\begin{aligned}
    & \CL_{\pi_0}(\CH,\CB) \\
    = & \min_{\delta\in \CB} \min_{h\in \CH} \max_{\lambda\geq 0} L(h, \delta, \lambda) \\
    \geq & \max_{\lambda\geq 0} \min_{\delta\in \CB} \min_{h\in \CH} L(h, \delta, \lambda) \\
    \delequal & \max_{\lambda\geq 0} \min_{\delta\in \CB} \min_{h\in \CH} \{h_{\pi_0}(x_0+\delta)-\lambda(f_{\pi_0}(x_0)-f^\sharp_{\pi_0}(x_0))\}\\
    = & \max_{\lambda\geq0} \min_{\delta\in\mathcal{B}} \{\lambda h^\sharp_{\pi_0}(x_0)-\int(\lambda\pi_0(z)-\pi_\delta(z))_+\mathrm{d}z\}
\nonumber
\end{aligned}
\end{equation}
where $\lambda$ is the Lagrangian multiplier. So all we need to do is to find such an interval $\mathcal{B}$, that  
\begin{equation}
\label{eq:cac>1/2}
    \max_{\lambda\geq0} \min_{\delta\in\mathcal{B}} \{\lambda h^\sharp_{\pi_0}(x_0)-\int(\lambda\pi_0(z)-\pi_\delta(z))_+\mathrm{d}z > \frac{1}{2}\}
\end{equation}
\end{theorem}

\noindent\textbf{Theorem 1. (binary case)} (restated) 
\textit{Let $\phi_S: \CW\times\BR\to \CW$ be the embedding transformation based on Staircase noise $\varepsilon \sim f_\gamma(w)$ and let $g_S$ be defined as the smoothed classifier as in (\ref{eq:smoothg1}). Suppose $y_A\in \CY$ and $\underline{p_A} \in (\frac{1}{2},1]$ satisfy: }
$$
    \BP(h(u\cdot \phi_S(w, \varepsilon))=y_A) \geq \underline{p_A}
$$
\textit{Then $g_S(u\cdot \phi_S(w, \delta_{\phi_S}))=y_A$ for all $\|\delta_{\phi_S}\|_1 \leq \rad_S\cdot\Delta$ where }
$$\rad_S=-\frac{1}{\epsilon}\log (2(1-\underline{p_A}))$$

\begin{proof}
Given the confidence lower bound
\begin{equation}
\begin{aligned}
    \CL_{\pi_0}(\CH,\CB)=&\max_{\lambda \geq 0} \min_{\|\delta\|_1\leq r} \{\lambda \underline{p_A}-\int(\lambda\pi_0(z)-\pi_\delta(z))_+ \rd z\} 
    % \\
    % =&\max_{\lambda \geq 0} \min_{\|\delta\|_?\leq r} \{\lambda \underline{p_A}-\int_{C_\lambda}(\lambda\pi_0(z)-\pi_\delta(z)) \rd z\}
\nonumber
\end{aligned}    
\end{equation}

According to Eq.(\ref{eq:f_gamma}), $\pi_0$ and $\pi_\delta$ are the staircase noise distributions as follows
\begin{equation}
\begin{aligned}\pi_0(z)=&f_\gamma^\epsilon(z)=\exp({-l_\Delta(z)\epsilon})a(\gamma), \\
\pi_{\delta}(z)=&f_\gamma^\epsilon(z+\delta)=\exp({-l_\Delta(z+\delta)\epsilon})a(\gamma),
\nonumber
\end{aligned}    
\end{equation}
where $l_\Delta(z+\delta)=\lfloor \frac{\|z+\delta\|_1}{\Delta}+(1-\gamma) \rfloor$.

As demonstrated in~\cite{zhang2020black}, the worst case for $\delta$ is obtained when $\delta^*=(r\cdot\Delta,0,\cdots,0)$, thus the bound is
\begin{equation}
\begin{aligned}
\label{eq:bound1}
    % \CL_{\pi_0}(\CH,\CB) \\
    % \max_{\lambda \geq 0} \{\lambda \underline{p_A}-& \int a(\gamma)(\lambda \exp({-l_\Delta(z)\epsilon}) -\exp({-l_\Delta(z+r\Delta)\epsilon})_+ \rd z\} \\
    \max_{\lambda \geq 0} & \{\lambda \underline{p_A}- \int a(\gamma)\exp({-l_\Delta(z_1)\epsilon}) \\
    &\quad [\lambda-\exp({(l_\Delta(z_1)-l_\Delta(z_1+r\Delta))\epsilon})]_+ \rd z_1\}
\end{aligned}    
\end{equation}

Denote $a$ to be the solution of the following equation
\begin{equation}
\begin{aligned}
    \lambda = \exp({[l_\Delta(a)-l_\Delta(a+r\Delta)]\epsilon}) \\
    \Longleftrightarrow \frac{\log \lambda}{\epsilon} = \frac{\|a\|_1-\|a+r\Delta\|_1}{\Delta}
\nonumber
\end{aligned}
\end{equation}

Then we have
% or $\frac{\log \lambda}{\epsilon} = \frac{|a_2|-|a_2+r|}{\Delta}-1$
$$ a =\left\{
\begin{aligned}
&-\infty, \quad& (\log \lambda)/\epsilon\geq r\\
&-\frac{\Delta}{2}(\frac{\log \lambda}{\epsilon}+r), \quad& -r < (\log \lambda)/\epsilon < r \\
&+\infty. \quad& (\log \lambda)/\epsilon\leq -r
\end{aligned}
\right.
$$ 
% or
% %
% $$
% a_2 =\left\{
% \begin{aligned}
% &-\infty, &\quad \Delta(\frac{\log \lambda}{\epsilon}+1)\geq r\\
% &-\frac{1}{2}(\Delta(\frac{\log \lambda}{\epsilon}+1)+r), &\quad -r < \Delta(\frac{\log \lambda}{\epsilon}+1) < r \\
% &+\infty. &\quad \Delta(\frac{\log \lambda}{\epsilon}+1)\leq -r
% \end{aligned}
% \right.
% $$ 

So the bound of $\int (\cdot)$ in Eq.(\ref{eq:bound1}) is 
\begin{equation}
\begin{aligned}
\label{eq:bound2}
    \lambda\int_{z_1>a}\exp&({-l_\Delta(z_1)\epsilon})a(\gamma)\rd z_1 \\
    & -\int_{z_1>a}\exp({-l_\Delta(z_1+\delta)\epsilon})a(\gamma)\rd z_1
% \nonumber
\end{aligned}
\end{equation}

\noindent\textbf{Case \rmnum{1})} $(\log \lambda)/\epsilon\geq r \Longleftrightarrow \lambda \geq \exp({r\epsilon})$

the bound is 
\begin{equation}
\label{eq:bound3}
    \max_{\lambda \geq \exp({r\epsilon})} \{\lambda \underline{p_A}-(\lambda-1)\}=1-\exp({r\epsilon}) (1-\underline{p_A})
\end{equation}

\noindent\textbf{Case \rmnum{2})} $-r < (\log \lambda)/\epsilon < r \Longleftrightarrow \exp({-r\epsilon}) < \lambda < \exp({r\epsilon})$

According to the formula for the summation of a geometric progression, we have the cumulative distribution function (CDF) of the staircase distribution as
%
% $$ F(x)=\int_x^{d\Delta} f(z) \rd z=\left\{
% \begin{aligned}
% &1-\frac{1}{2} \frac{1-\exp({\frac{x}{\Delta}\epsilon})}{1-\exp({-d\epsilon})}, \quad& x < 0 \\
% &\frac{1}{2} \frac{1-\exp({-\frac{x}{\Delta}\epsilon})}{1-\exp({-d\epsilon})}, \quad& x\geq 0
% \end{aligned}
% \right. =>
% $$ 
%
$$ \int_\mu^{d\Delta} f_\gamma^\epsilon(z) \rd z=\left\{
\begin{aligned}
&1-\frac{1}{2} \frac{1-\exp({(\frac{\mu}{\Delta}+s)\epsilon})}{1-\exp({s\epsilon})}, &\mu < 0 \\
&\frac{1}{2} \frac{1-\exp({(-\frac{\mu}{\Delta}+s)\epsilon})}{1-\exp({s\epsilon})}, &\mu\geq 0
\end{aligned}
\right.
$$ 
where $s$ is the total number of stairs that is greater than 0.

Thus, the bound is 
\begin{equation}
\begin{aligned}
    & \CL_{\pi_0}(\CH,\CB) \\
    =& \max_{\lambda}\{\lambda \underline{p_A} - \lambda[1-\frac{1}{2}\frac{1-\exp({(\frac{a}{\Delta}+s)\epsilon})}{1-\exp({s\epsilon})}] \\
    &\qquad \qquad \qquad \quad +\frac{1}{2}\frac{1-\exp({[-(\frac{a}{\Delta}+r)+s]\epsilon})}{1-\exp({s\epsilon})}\} \\
    =& \max_{\lambda}\{\lambda (\underline{p_A}-1)+\frac{\lambda}{2}\frac{1-\exp({-\frac{1}{2}(\log \lambda+r\epsilon)}) \exp({s\epsilon})}{1-\exp({s\epsilon})} \\
    &\qquad \qquad \qquad \quad +\frac{1}{2}\frac{1-\exp({\frac{1}{2}(\log \lambda-r\epsilon)})\exp({s\epsilon})}{1-\exp({s\epsilon})}\}
    % =& 1-\exp({r\epsilon}) (1-\underline{p_A})
\nonumber
\end{aligned}
\end{equation}

Next, we analyze how to obtain the actual bound. We can rewrite the bound function of the second equation above as follows
% In order to obtain the extremum of the bound
\begin{equation}
\begin{aligned}
\CL_{\pi_0}(\CH,\CB)=& \max_{\lambda}\{ c_1\cdot \lambda+\lambda\cdot\frac{1-c_3\cdot \exp({-\frac{1}{2}\log \lambda})}{c_2} \\
&\qquad \qquad \quad +\frac{1-c_3\cdot \exp({\frac{1}{2}\log \lambda})}{c_2} \} \\
=& \max_{\lambda}\{\dfrac{ (c_1 c_2+1) \lambda -2c_3\sqrt{\lambda}+1}{c_2} \}
\nonumber
\end{aligned}
\end{equation}
where $c_1=\underline{p_A}-1\in(-\frac{1}{2}, 0),\ c_2=2(1-\exp({s\epsilon}))<0,\ c_3=\exp({(s-\frac{r}{2}})\epsilon)>\exp(\frac{s\epsilon}{2})$. We derive the derivative for $\lambda$ and obtain that the extremum is achieved when 
\begin{equation}
\begin{aligned}
    \frac{\partial \CL_{\pi_0}(\CH,\CB)}{\partial \lambda} & = \dfrac{-\frac{c_3}{\sqrt{\lambda}}+c_1c_2+1}{c_2} = 0 \\
    \Longleftrightarrow \sqrt{\hat{\lambda}} & = \frac{c_3}{1+c_1 c_2}
\nonumber
\end{aligned}
\end{equation}

We notice that $\exp(-r\epsilon) < \hat{\lambda} < \exp(r\epsilon)$ all the time. So during the interval $\lambda \in (\exp({-r\epsilon}),\exp({r\epsilon}))$, the bound is 
\begin{equation}
\label{eq:bound4}
    \CL_{\pi_0}(\CH,\CB) \Big|_{\lambda=\hat{\lambda}} = \frac{1}{c_2} (1-\frac{(c_3)^2}{1+c_1c_2}).
\end{equation}

However, the bound in Eq.(\ref{eq:bound4}) is less than $\frac{1}{2}$ all the time, which does not satisfy the condition in Eq.(\ref{eq:cac>1/2}), i.e., 
\begin{equation}
\begin{aligned}
\label{eq:bound4_2}
    \CL_{\pi_0}(\CH,\CB)\Big|_{\lambda=\hat{\lambda}} < \frac{1}{2} \Longleftrightarrow \qquad &\\
    \exp(\frac{1}{2} r\epsilon) [1+2(1-p_A)(\exp(s\epsilon)-1)] & > 1.
% \nonumber
\end{aligned}
\end{equation}

% The function $\partial \CL_{\pi_0}(\CH,\CB)/ \partial \lambda$ is a decreasing function due to $-c_3/c_2>0$. 
% the value of $\partial \CL_{\pi_0}(\CH,\CB)/ \partial \lambda$ is either consistently less than 0 or negative ($<0$) and then positive ($>0$).
%
% \begin{equation}
% \begin{aligned}
% \frac{\partial \CL_{\pi_0}(\CH,\CB)}{\partial \lambda}
% =&\frac{1-\exp({s\epsilon -\frac{1}{2}(r\epsilon+\log \lambda)})}{2[1-\exp({s \epsilon})]}+c_1 \\
% \in& (c_1+\frac{1-\exp({(s-r)\epsilon})}{2[1-\exp(s \epsilon)]}, c_1+\frac{1}{2})
% \nonumber
% \end{aligned}
% \end{equation}

% \noindent\ding{172} $\lambda = (\frac{c_3}{1+c_1 c_2})^2$, if the extremum 
% $\hat{\lambda} < \exp(r\epsilon)$ 
% \begin{equation}
% \begin{aligned}
%     \Longleftrightarrow \underline{p_A} &< 1-\frac{\exp((s-r)\epsilon)-1}{2[\exp(s \epsilon)-1]} \\
%     \Longleftrightarrow \exp(\frac{3r}{2s}) &> \frac{1}{1+2(1-p_A)(\exp(5)-1)}
% \nonumber
% \end{aligned}
% \end{equation}

% \noindent\ding{173} $\lambda = \exp(r\epsilon)$, if the extremum $\hat{\lambda} \geq \exp(r\epsilon)$ 
% $$\Longleftrightarrow \underline{p_A} \geq 1-\frac{\exp((s-r)\epsilon)-1}{2[\exp(s \epsilon)-1]}$$.

% Thus the actual bound in Case \rmnum{2}) is
% \begin{equation}
% \label{eq:bound4}
%     1-\exp({r\epsilon}) (1-\underline{p_A}).
% \end{equation}

\noindent\textbf{Case \rmnum{3})} $(\log \lambda)/\epsilon\leq -r \Longleftrightarrow \lambda \leq \exp({-r\epsilon})$

the bound is
\begin{equation}
\label{eq:bound5}
    \max_{\lambda \leq \exp({-r\epsilon})} \lambda \underline{p_A}=\exp({-r\epsilon}) \underline{p_A}.
\end{equation}

Combining the above bound Eq.(\ref{eq:bound3}), Eq.(\ref{eq:bound4_2}), Eq.(\ref{eq:bound5}) in three cases, the final bound is 
\begin{equation}
\label{eq:bound6}
    \max(\exp({-r\epsilon}) \underline{p_A}, 1-\exp({r\epsilon}) (1-\underline{p_A})).
\end{equation}

Since $\exp({-r\epsilon}) \underline{p_A} > 1-\exp({r\epsilon}) (1-\underline{p_A}) \Longleftrightarrow \underline{p_A}<\frac{1}{1+\exp({-r\epsilon})}$, Eq.(\ref{eq:bound6}) can be rewrite as
\begin{equation}
\label{eq:bound7}
\left\{
\begin{aligned}
&\exp({-r\epsilon}) \underline{p_A}, &\quad \underline{p_A}<\frac{1}{1+\exp({-r\epsilon})}\\
&1-\exp({r\epsilon}) (1-\underline{p_A}). &\quad \mathrm{otherwise} 
\end{aligned}
\right.
\end{equation}

Actually, in the first case, when $\underline{p_A}<\frac{1}{1+\exp({-r\epsilon})}$, we have the confidence lower bound $\exp({-r\epsilon}) \underline{p_A}< 1-\underline{p_A} <\frac{1}{2}$ all the time.
\end{proof}

\begin{remark}
When $\ \underline{p_A}\geq\frac{1}{1+\exp({-r\epsilon})}$,  the radius bound is 
$$ %\left\{
\begin{aligned}
% \exp({-r\epsilon}) \underline{p_A} > \frac{1}{2} &\Longleftrightarrow r < \frac{\log (2\underline{p_A})}{\epsilon}, &\ \underline{p_A}<\frac{1}{1+\exp({-r\epsilon})}\\
1-\exp({r\epsilon}) (1-\underline{p_A})> \frac{1}{2} &\Longleftrightarrow r < -\frac{1}{\epsilon}\log (2(1-\underline{p_A})).
\end{aligned}
% \right.
$$
When $\underline{p_A}<\frac{1}{1+\exp({-r\epsilon})}$, the radius bound is $r=0$.
% Actually, we have $\frac{\log (2\underline{p_A})}{\epsilon}<-\frac{\log (2(1-\underline{p_A}))}{\epsilon}$ all the time.
\end{remark}

%%%%%%%%%%%%%%%%%%%%%%%%%%%%%%%%%%%%%%%%%%%%%%%%%%%%%%%%%%%%%%%%%%%%%%%%%%%%%%%%

\section{Proof for Multiplicative Noise}

\subsection{Proof for Theorem 2}
\textbf{Staircase Distribution}

According to our definition in Eqn.~\ref{eq:h_gamma}, we have:
$\pi_0$ has the staircase distribution and 
$$\pi_0(z)=e^{-h_\gamma(z)\varepsilon}a(\gamma), \pi_{\delta}(z)=e^{-h_{\delta\gamma}(z)\varepsilon}a(\delta\gamma).$$
where $h_{\delta\gamma}(x)=\lfloor \frac{x}{\Delta}+(1-\delta\gamma) \rfloor$.

$$\pi_0(z)=e^{-h_\gamma(z)\varepsilon}a(\gamma), \pi_{\delta}(z)=e^{-h_{\gamma}(z+\delta)\varepsilon}a(\gamma).$$
where $h_{\gamma}(x+\delta)=\lfloor \frac{x+\delta}{\Delta}+(1-\gamma) \rfloor$.

In order to calculate $\int(\lambda \pi_0(z)-\pi_\delta(z))_+\rd z=\int_{C_\lambda}(\lambda \pi_0(z)-\pi_\delta(z))\rd z$. 
Let 
\begin{equation}
\begin{aligned}
    C_\lambda:=&\{z:\lambda\pi_0(z)\geq\pi_\delta(z)\} \\
    =&\{z:-h_\gamma(z)\epsilon+\log \lambda \geq -h_{\gamma}(z+\delta)\epsilon\} \\
    =&\{z:h_{\gamma}(z+\delta)-h_\gamma(z)\geq -\frac{\log \lambda}{\epsilon} \} \\
    =&\{ \lfloor \frac{|z+\delta|}{\Delta}+(1-\gamma) \rfloor - \lfloor \frac{|z|}{\Delta}+(1-\gamma) \rfloor \geq -\frac{\log \lambda}{\epsilon}\}
\nonumber
\end{aligned}
\end{equation}

\begin{figure*}[] %H为当前位置，!htb为忽略美学标准，htbp为浮动图形
\centering
\includegraphics[width=0.8\linewidth]{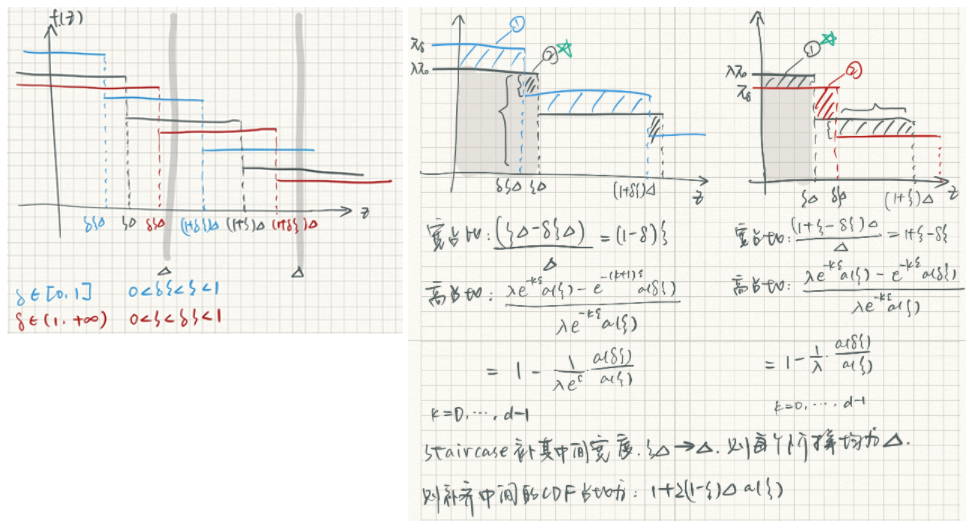} 
\caption{staircase mechanism with different $\delta$} 
\label{fig:staircase_delta} 
\end{figure*}

According to $h_{\delta\gamma}(z)-h_\gamma(z)=\lfloor \frac{x}{\Delta}+(1-\delta\gamma) \rfloor-\lfloor \frac{x}{\Delta}+(1-\gamma) \rfloor\in \{-1,0,1\}$, we discuss $C_\lambda$ by case

\noindent $\blacksquare$ 1) When $\delta\in(0,1]$ as Figure~\ref{}, we have $h_{\delta\gamma}(z)-h_\gamma(z)\in \{0,1\}$

(i) $\frac{1}{\epsilon}(\log a(\delta\gamma)-\log\lambda a(\gamma))\in(-\infty,0] \Leftrightarrow \lambda\geq\dfrac{a(\delta\gamma)}{a(\gamma)}$, then $C_\lambda=(-\infty, +\infty)$. 

the bound is
\begin{equation}
\begin{aligned}
    \CL_{\pi_0}(\CF,\CB)&=\min_{\delta\in\mathcal{B}}\max_{\lambda\geq\dfrac{a(\delta\gamma)}{a(\gamma)}}\{\lambda f^\#_{\pi_0}(x_0)-\int_{C_\lambda}(\lambda\pi_0(z)-\pi_\delta(z)) \mathrm{d}z\} \\
    &=\min_{\delta\in\mathcal{B}}\max_{\lambda\geq\dfrac{a(\delta\gamma)}{a(\gamma)}}\{\lambda p_A-(\lambda-1)\} \\
    &=\min_{\delta\in\mathcal{B}}\{1-\dfrac{a(\delta\gamma)}{a(\gamma)}(1-p_A)\} 
\nonumber
\end{aligned}
\end{equation}

(ii) $\frac{1}{\epsilon}(\log a(\delta\gamma)-\log\lambda a(\gamma))\in(0,1] \Leftrightarrow \dfrac{a(\delta\gamma)-e^\epsilon}{a(\gamma)}\leq\lambda<\dfrac{a(\delta\gamma)}{a(\gamma)}$

$\bigcap \lambda\geq 0$, we have $0\leq\lambda<\dfrac{a(\delta\gamma)}{a(\gamma)}$

then $C_\lambda=\{z:h_{\delta\gamma}(z)-h_\gamma(z)=1\}=\{z:(k+\delta\gamma)\Delta<z\leq(k+\gamma)\Delta\}$, $k\in[-d,d)$ and $k\in \BZ$, i.e., the black 2 in Figure~\ref{}. 

the bound is 
% \overset{def}{=}
\begin{equation}
\begin{aligned}
\mathcal{L}_{\pi_0}(\mathcal{F},\mathcal{B})&\overset{(1)}{=}\min_{\delta\in\mathcal{B}}\max_{\lambda}\{\lambda p_A- \\
&\qquad \lambda[1+2(1-\gamma)\Delta a(\gamma)] (1-\delta)\gamma\cdot(1-\dfrac{1}{\lambda e^\epsilon}\dfrac{a(\delta\gamma)}{a(\gamma)})\} \\
&=\min_{\delta\in\mathcal{B}}\max_{\lambda}\{\lambda p_A-t_1(1-\delta)(\lambda-\dfrac{a(\delta\gamma)}{e^\epsilon a(\gamma)})\} \\
&\overset{(2)}{=}\min_{\delta\in\mathcal{B}} \{\dfrac{p_A}{e^\epsilon} \dfrac{a(\delta\gamma)}{a(\gamma)}>\dfrac{1}{2}\} 
\nonumber
\end{aligned}
\end{equation}
where $t_1=[1+2(1-\gamma)\Delta a(\gamma)]\gamma>0$ is a constant.

For equation (1) we use the proportional method to calculate $\int_{C_\lambda}(\lambda\pi_0(z)-\pi_\delta(z)) \rd z$. Firstly, we expand the length of the first staircase from $2\gamma\Delta$ to the length of $2\Delta$. So the area of the whole PDF function is expanded by $[1+2(1-\gamma)\Delta a(\gamma)]\times$ the original area.
Secondly, for each $k$, the area of black 2 can be converted to a certain proportion of the area of gray. The length and width of black 2 are $l_1$ and $w_1$ of gray, respectively.
\begin{equation}
\begin{aligned}
l_1&=(1-\delta)\gamma, \\
w_1&=\dfrac{\lambda e^{-k\epsilon}a(\gamma)-e^{-(k+1)\epsilon}a(\delta\gamma)}{\lambda e^{-k\epsilon}a(\gamma)}=1-\dfrac{1}{\lambda e^\epsilon}\dfrac{a(\delta\gamma)}{a(\gamma)}
\nonumber
\end{aligned}
\end{equation}

For equation (2), we calculate the $\frac{\partial \mathcal{L}}{\partial \lambda}$. 

\ding{172}$\frac{\partial \mathcal{L}}{\partial \lambda}=0 \Leftrightarrow \delta=1-\dfrac{p_A}{t_1}$, then
\begin{equation}
\CL_{\pi_0}(\CF,\CB)=\min_{\delta\in\CB} \{\dfrac{p_A}{e^\epsilon} \dfrac{a(\delta\gamma)}{a(\gamma)}\}
\nonumber
\end{equation}

\ding{173}$\frac{\partial \mathcal{L}}{\partial \lambda}>0 \Leftrightarrow \delta>1-\dfrac{p_A}{t_1}$, then
\begin{equation}
\begin{aligned}
\CL_{\pi_0}(\CF,\CB)&=\min_{\delta\in\CB}\{\dfrac{a(\delta\gamma)}{a(\gamma)} [p_A- t(1-\delta)(1-\dfrac{1}{e^\epsilon})]\} \\
&>\min_{\delta>1-\dfrac{p_A}{t}}\{\dfrac{p_A}{e^\epsilon}\dfrac{a(\delta\gamma)}{a(\gamma)}\}
\nonumber
\end{aligned}
\end{equation}
the first extremum is achieved when $\lambda=\dfrac{a(\delta\gamma)}{a(\gamma)}$. the second extremum is achieved when $\delta=1-\dfrac{p_A}{t_1}$. 

\ding{174}$\frac{\partial \mathcal{L}}{\partial \lambda}<0 \Leftrightarrow \delta<1-\dfrac{p_A}{t_1}$, then
\begin{equation}
\begin{aligned}
\CL_{\pi_0}(\CF,\CB)&=\min_{\delta\in\CB}\{t(1-\delta)\dfrac{a(\delta\gamma)}{e^\epsilon a(\gamma)}\}\\
&>\min_{\delta<1-\dfrac{p_A}{t}}\{\dfrac{p_A}{e^\epsilon}\dfrac{a(\delta\gamma)}{a(\gamma)}\}
\nonumber
\end{aligned}
\end{equation}
the first extremum is achieved when $\lambda=0$. the second extremum is achieved when $\delta=1-\dfrac{p_A}{t_1}$.

(iii)$\frac{1}{\epsilon}(\log a(\delta\gamma)-\log\lambda a(\gamma))\in(1,\infty) \Leftrightarrow \lambda < \dfrac{a(\delta\gamma)-e^\epsilon}{a(\gamma)}$
$\bigcap \lambda\geq 0$, we have $\lambda\in \emptyset$.

\textbf{Remark 1.} When $\delta\in (0, 1]$, the bound is
\begin{equation}
\CL_{\pi_0}(\CF,\CB)=\min_{\delta\in\CB}
\left\{  
\begin{aligned}
    \dfrac{p_A}{e^\epsilon}\dfrac{a(\delta\gamma)}{a(\gamma)} &,\qquad 0\leq\lambda<\dfrac{a(\delta\gamma)}{a(\gamma)}    \\
    1-\dfrac{a(\delta\gamma)}{a(\gamma)}(1-p_A) &,\qquad \lambda\geq\dfrac{a(\delta\gamma)}{a(\gamma)}
\end{aligned}
\right.  
\label{eq:delta_1}
\end{equation}

\noindent $\blacksquare$ 2) When $\delta\in (1,\frac{1}{\gamma})$ as Figure~\ref{}, we have $h_{\delta\gamma}(z)-h_\gamma(z)\in\{-1,0\}$.

(i) $\frac{1}{\epsilon}(\log a(\delta\gamma)-\log\lambda a(\gamma))\in(-\infty,-1] \Leftrightarrow \lambda\geq\dfrac{a(\delta\gamma)+e^\epsilon}{a(\gamma)}$, then $C_\lambda=(-\infty,+\infty)$.

the bound is 
\begin{equation}
\begin{aligned}
    \CL_{\pi_0}(\CF,\CB)&=\min_{\delta\in\CB}\max_{\lambda\geq\dfrac{a(\delta\gamma)+e^\epsilon}{a(\gamma)}}\{\lambda p_A-(\lambda-1)\} \\
    &=\min_{\delta\in\CB}\{1-\dfrac{a(\delta\gamma)+e^\epsilon}{a(\gamma)}(1-p_A)\}
\nonumber
\end{aligned}
\end{equation}

(ii) $\frac{1}{\epsilon}(\log a(\delta\gamma)-\log\lambda a(\gamma))\in(-1,0] \Leftrightarrow \dfrac{a(\delta\gamma)}{a(\gamma)} \leq \lambda< \dfrac{a(\delta\gamma)+e^\epsilon}{a(\gamma)}$

then $C_\lambda=\{z: h_{\delta\gamma}(z)-h_\gamma(z)=0\}=\{z:(k+\delta\gamma)\Delta<z\leq(k+1+\gamma)\Delta\}$, $k\in[-d,d)$ and $k\in\BZ$, i.e., the black 1 in Figure~\ref{}.

the bound is
\begin{equation}
\begin{aligned}
    \mathcal{L}_{\pi_0}(\mathcal{F},\mathcal{B})&\overset{(1)}{=}\min_{\delta\in\CB}\max_{\lambda}\{\lambda p_A- \\
    &\lambda[1+2(1-\gamma)\Delta a(\gamma)][1+(1-\delta)\gamma](1-\dfrac{a(\delta\gamma)}{\lambda a(\gamma)})\} \\
    &\overset{(2)}{=}\min_{\delta\in\CB}\max_{\lambda}\{\lambda p_A-t_1[1+(1-\delta)\gamma](\lambda-\dfrac{a(\delta\gamma)}{a(\gamma)})\}
\nonumber
\end{aligned}
\end{equation}
where $t_2=[1+2(1-\gamma)\Delta a(\gamma)]>1$ is a constant.

As in the proof of setting 1) (ii). For equation (1), the length and width of black 1 are $l_2$ and $w_2$ of gray, respectively.
\begin{equation}
\begin{aligned}
l_2&=1+\gamma-\delta\gamma, \\
w_2&=\dfrac{\lambda e^{-k\epsilon}a(\gamma)-e^{-k\epsilon}a(\delta\gamma)}{\lambda e^{-k\epsilon}a(\gamma)}=1-\dfrac{1}{\lambda}\dfrac{a(\delta\gamma)}{a(\gamma)}
\nonumber
\end{aligned}
\end{equation}

For equation (2), we calculate the $\frac{\partial \mathcal{L}}{\partial \lambda}$

\ding{172}$\frac{\partial \mathcal{L}}{\partial \lambda}=0 \Leftrightarrow \delta=1+\dfrac{t_2-p_A}{t_2\gamma}=1+\dfrac{1}{\gamma}-\dfrac{p_A}{t_2\gamma}$, then
\begin{equation}
\CL_{\pi_0}(\CF,\CB)=\min_{\delta\in\CB} \{p_A\dfrac{a(\delta\gamma)}{a(\gamma)}\}
\nonumber
\end{equation}

\ding{173}$\frac{\partial \mathcal{L}}{\partial \lambda}>0 \Leftrightarrow \delta>1+\dfrac{1}{\gamma}-\dfrac{p_A}{t_2\gamma}$, then
\begin{equation}
\begin{aligned}
    \mathcal{L}_{\pi_0}(\mathcal{F},\mathcal{B})&=\min_{\delta\in \CB}\{\dfrac{a(\delta\gamma)}{a(\gamma)}p_A+\dfrac{e^\epsilon}{a(\gamma)}(p_A-t_2[1+(1-\delta)\gamma])\} \\
    &>\min_{\delta>1+\dfrac{1}{\gamma}-\dfrac{p_A}{t_2\gamma}}\{p_A\dfrac{a(\delta\gamma)}{a(\gamma)}\}
\nonumber
\end{aligned}
\end{equation}
the first extremum is achieved when $\lambda = \dfrac{a(\delta\gamma)+e^\epsilon}{a(\gamma)}$, the second extremum is achieved when $\delta=1+\dfrac{1}{\gamma}-\dfrac{p_A}{t_2\gamma}$.

\ding{174}$\frac{\partial \mathcal{L}}{\partial \lambda}<0 \Leftrightarrow \delta<1+\dfrac{1}{\gamma}-\dfrac{p_A}{t_2\gamma}$, then
$$\mathcal{L}_{\pi_0}(\mathcal{F},\mathcal{B})>\min_{\delta<1+\dfrac{1}{\gamma}-\dfrac{p_A}{t_2\gamma}}\{p_A\dfrac{a(\delta\gamma)}{a(\gamma)}\}$$
the extremum is achieved when $\lambda = \dfrac{a(\delta\gamma)}{a(\gamma)}, \delta=1+\dfrac{1}{\gamma}-\dfrac{p_A}{t_2\gamma}$.

(iii) $\frac{1}{\epsilon}(\log a(\delta\gamma)-\log\lambda a(\gamma))\in(0,\infty)\Leftrightarrow \lambda < \dfrac{a(\delta\gamma)}{a(\gamma)}$
$\bigcap \lambda\geq 0$, we have $0\leq\lambda<\dfrac{a(\delta\gamma)}{a(\gamma)}$
, then $C_\lambda=\emptyset$

the bound is
$$\mathcal{L}_{\pi_0}(\mathcal{F},\mathcal{B})=\min_{\delta\in\mathcal{B}}\max_{\lambda\geq0}\{\lambda p_A\}> \min_{\delta\in\CB}\{p_A\dfrac{a(\delta\gamma)}{a(\gamma)}\} $$

\textbf{Remark 2.} When $\delta\in (1,\frac{1}{\gamma})$, the bound is
\begin{equation}
\CL_{\pi_0}(\CF,\CB)=\min_{\delta\in\CB}
\left\{  
\begin{aligned}
    p_A\dfrac{a(\delta\gamma)}{a(\gamma)} &,\ 0\leq\lambda<\dfrac{a(\delta\gamma)+e^\epsilon}{a(\gamma)}    \\
    1-\dfrac{a(\delta\gamma)+e^\epsilon}{a(\gamma)}(1-p_A) &,\ \lambda\geq\dfrac{a(\delta\gamma)+e^\epsilon}{a(\gamma)}
\end{aligned}
\right.  
\label{eq:delta_2}
\end{equation}

According to Eqn.\ref{eq:delta_1} and Eqn.\ref{eq:delta_2}, we need to calculate the maximum and minimum of $\dfrac{a(\delta\gamma)}{a(\gamma)}$ to calculate $\CB$, so we define 
\begin{equation}
\begin{aligned}
    G(\delta)&=\dfrac{a(\delta\gamma)}{a(\gamma)}=\dfrac{\sum_{k=1}^d \tbinom{d}{k}c_{d-k}(b+(1-b)\gamma^k)}{\sum_{k=1}^d \tbinom{d}{k}c_{d-k}(b+(1-b)(\delta\gamma)^k)} \\
    &=\dfrac{C_1}{C_2+C_3\sum_{k=1}^d \delta^k}
\end{aligned}
\label{eq:G(delta)}
\end{equation}
where $C_1,C_2,C_3 >0$

$G'(\delta)=-\dfrac{C_1 C_3\sum_{k=1}^d k\delta^{k-1}}{(C_2+C_3\sum_{k=1}^d \delta^k)^2} <0, \forall \delta$

when $\delta\in(0,1]$, we define $\delta_1,\delta_2\in(0,1]$ as: $\dfrac{p_A}{e^\epsilon}G(\delta_1)=\dfrac{1}{2}$ and $1-G(\delta_2)(1-p_A)=\dfrac{1}{2}$, then $\delta\in (0,\delta_1)\cap (\delta_2,1]$.

when $\delta\in(1,\dfrac{1}{\gamma}]$, we define $\delta_3,\delta_4\in(1,\dfrac{1}{\gamma}]$ as: $p_A G(\delta_3)=\dfrac{1}{2}$ and $1-(G(\delta_4)+\dfrac{e^\epsilon}{a(\gamma)})(1-p_A)=\dfrac{1}{2}$, then $\delta\in (1,\delta_3)\cap (\delta_4,\dfrac{1}{\gamma}]$

If there is no eligible $\delta_i$, delete the interval corresponding to the value of $\delta_i$.

\subsection{Proof for Theorem 3}

The assumption is 
\begin{equation}
    \BP((f\circ \psi_\beta)(x)=y_A)=p_A\geq\underline{p_A}\geq \overline{p_B} \geq p_B=\BP((f\circ \psi_\beta)(x)=y_B)
\nonumber
\end{equation}

By the definition of $g$, we need to show that 
\begin{equation}
    \BP((f\circ \psi_{\beta\delta})(x)=y_A) \geq \BP((f\circ \psi_{\beta\delta})(x)=y_B)
\nonumber
\end{equation}

We define the set $A, B$ to satisfy the following inequalities

\begin{equation}
\begin{aligned}
    \BP ((f \circ \psi_{\beta\delta})(x)=y_A)\overset{(1)}{\geq} \BP(\beta\delta\in A) \\
    \overset{(2)}{>} \BP(\beta\delta\in B) \overset{(3)}{\geq}\BP((f \circ \psi_{\beta\delta})(x)=y_B)
\nonumber
\end{aligned}
\end{equation}
for all $\delta\in(\delta_1,\delta_2)$, where 
$$A=\{z|z\leq xxx\}, B=\{z|z\geq xxx\}$$

$\delta \geq 1 ??? $

(1) Assume $p_\beta(z)$ is the PDF of random variable $\beta$. Then
\begin{equation}
\begin{aligned}
     &\BP(f\circ \psi_{\beta\delta}(x)=y_A)-\BP(\beta\delta\in A) \\
    =&\int_\BR [f\circ \psi_z(x)=y_A]p_{\beta\delta}(z)\rd z-\int_A p_{\beta\delta}(z)\rd z \\
    =&(\int_{\BR\backslash A}[f\circ \psi_z(x)=y_A]p_{\beta\delta}(z)\rd z + \int_A [f\circ \psi_z(x)=y_A]p_{\beta\delta}(z)\rd z) \\
    &-(\int_A [f\circ \psi_z(x)=y_A]p_{\beta\delta}(z)\rd z+ \int_A [f\circ \psi_z(x)\neq y_A]p_{\beta\delta}(z)\rd z) \\
    =&\int_{\BR \backslash A}[f \circ \psi_z(x)=y_A]p_{\beta\delta}(z)\rd z-\int_A[f\circ \psi_z(x)\neq y_A]p_{\beta\delta} (z)\rd z \\
    \overset{Lemma 6}{\geq}& t(\int_{\BR \backslash A}[f \circ \psi_z(x)=y_A]p_{\beta}(z)\rd z-\int_A[f\circ \psi_z(x)\neq y_A]p_\beta (z)\rd z) \\
    =& t(\int_{\BR}[f \circ \psi_z(x)=y_A]p_{\beta}(z)\rd z-\int_A p_\beta(z)\rd z) \\
    =& t(p_A-\underline{p_A}) \geq 0
\nonumber
\end{aligned}
\end{equation}

For $\beta \sim \mathrm{Staircase}(\gamma)$, and $\beta\delta \sim \mathrm{Staircase}(\delta\gamma)$, we have $\gamma\in[0,1]$ and $\delta\gamma\in[0,1] \Leftrightarrow \delta\in[0,\frac{1}{\gamma}]$.

\textbf{Lemma 6.} There exists $t > 0$ such that $p_{\beta\delta}(z) \leq t\cdot p_{\beta}(z)$ for all $z \in A$. And further $p_{\beta\delta}(z) > t\cdot p_\beta(z)$ for all $z \in \BR \backslash A$.

\begin{proof}
change line\\

$\dfrac{p_{\beta \delta}(z)}{p_\beta (z)}=\dfrac{f_{\delta\gamma}(z)}{f_\gamma(z)}=\dfrac{e^{-h_{\beta\gamma}(x)\varepsilon}a(\delta\gamma)}{e^{-h_\gamma(x)\varepsilon}a(\gamma)}=e^{(h_\gamma(z)-h_{\delta\gamma}(z))\varepsilon}G(\delta)$, 
where $G(\delta)=\dfrac{a(\delta\gamma)}{a(\gamma)}$ and $G'(\delta)<0, \forall \delta$ from Eqn.~\ref{eq:G(delta)}.

What is the lowest $t$ if it exists such that $\dfrac{p_{\beta \delta}(z)}{p_\beta (z)} \leq t$ ? $\Leftrightarrow$ find the maximum value of $\dfrac{p_{\beta \delta}(z)}{p_\beta (z)}$ when $z \in A$

\noindent $\blacksquare$ When $\delta\in(0,1]$, we have $h_\gamma(z)-h_{\delta\gamma}(z)\in \{-1,0\}$. 

$h_\gamma(z)-h_{\delta\gamma}(z)=0 \Leftrightarrow z\in[k\Delta ,(k+\delta\gamma)\Delta], k\in[-d,d)$, i.e., the blue 1. Then
$$\dfrac{p_{\beta \delta}(z)}{p_\beta (z)}=G(\delta)$$

$h_\gamma(z)-h_{\delta\gamma}(z)=-1 \Leftrightarrow z\in[(k+\delta\gamma)\Delta,(k+\gamma)\Delta], k\in[-d,d)$, i.e., the black 2. Then
$$\dfrac{p_{\beta \gamma}(z)}{p_\beta (z)}=e^{-\varepsilon} G(\delta)$$

i) when $A=\{z|(k+\delta\gamma)\Delta \leq z \leq (k+\gamma)\Delta, k\in[-d,d)\}$, the lowest $t$ is
$$t=e^{-\varepsilon}G(\delta)=e^{-\varepsilon}G(\delta_1), \delta_1\in(0,1)$$

ii) when $A=(-\infty,\infty)$, the lowest $t$ is
$$t=G(\delta)=G(1), \delta_2\in(0,1)$$

\noindent $\blacksquare$ When $\delta\in(1,\frac{1}{\gamma}]$, we have $h_\gamma(z)-h_{\delta\gamma}(z)\in \{0,1\}$.

$h_\gamma(z)-h_{\delta\gamma}(z)=0 \Leftrightarrow z\in[k\Delta,(k+\gamma)\Delta], k\in[-d,d)$, i.e., the black 1. Then
$$\dfrac{p_{\beta \delta}(z)}{p_\beta (z)}=G(\delta)$$

$h_\gamma(z)-h_{\delta\gamma}(z)=1 \Leftrightarrow z\in[(k+\gamma)\Delta,(k+\delta\gamma)\Delta], k\in[-d,d)$, i.e., the red 2. Then
$$\dfrac{p_{\beta \delta}(z)}{p_\beta (z)}=e^\varepsilon G(\delta)$$ 

i) when $A=\{z|k\Delta \leq z \leq (k+\gamma)\Delta, k\in[-d,d)\}$, the lowest $t$ is
$$t=G(\delta)=G(\delta_3), \delta_3\in(1,\frac{1}{\gamma})$$

ii) when $A=(-\infty,\infty)$, the lowest $t$ is
$$t=e^\varepsilon G(\delta)=e^\varepsilon G(\frac{1}{\gamma}), \delta_4\in(1,\frac{1}{\gamma})$$

\end{proof}
